# Supplementary material for: Defending From Physically-Realizable Adversarial Attacks Through Internal Over-Activation Analysis
Source: arXiv:2203.07341 source file (2022-09-15)
Supplement: Supplementary file 1 [file appendix.tex]

\section{Supplementary Material for ''TITLE"}
